# Supplementary material for: Nowhere to Hide: Radio-faint AGN in the GOODS-N field. I. Initial catalogue and radio properties
Source: arXiv:1808.04296 source file (2018-08-15)
Supplement: Supplementary file 1 [file source_cataloguing_appendix.tex]

\section{Source cataloguing}~\ref{Appendix:source_cataloguing}
